# Supplementary material for: Modifying the Optical Emission of Vanadyl Phthalocyanine via Molecular Self-Assembly on van der Waals Materials
Source: arXiv:2509.05438 ancillary file (2025-09-05)
Supplement: Supplementary file 1 [file Gavin_2025_SI.pdf]

# Supplemental Information: Modifying the Optical Emission of Vanadyl Phthalocyanine via Molecular Self-assembly on van der Waals Materials

S. Carin Gavin,<sup>1,\*</sup> William Koll,<sup>2,\*</sup> Moumita Kar,<sup>3,\*</sup> Yiyang Liu,<sup>1</sup> Anushka Dasgupta,<sup>4</sup> Ethan Garvey,<sup>1</sup> Thomas W. Song,<sup>4</sup> Chunxi Zhou,<sup>1</sup> Brendan P. Kerwin,<sup>3</sup> Jash Jain,<sup>1</sup> Tobin J. Marks,<sup>3,4,5,6</sup> Mark C. Hersam,<sup>3,4,6,7</sup> George C. Schatz,<sup>3</sup> Jay A. Gupta,<sup>2</sup> and Nathaniel P. Stern<sup>1,†</sup>

<sup>1</sup>*Department of Physics and Astronomy, Northwestern University, Evanston, IL 60208, USA*

<sup>2</sup>*Department of Physics, The Ohio State University, Columbus, Ohio 43210, USA*

<sup>3</sup>*Department of Chemistry, Northwestern University, Evanston, IL 60208, USA*

<sup>4</sup>*Department of Materials Science and Engineering,  
Northwestern University, Evanston, IL 60208, USA*

<sup>5</sup>*Department of Chemical and Biological Engineering,  
Northwestern University, Evanston, IL 60208, USA*

<sup>6</sup>*Materials Research Center, Northwestern University, Evanston, IL 60208, USA*

<sup>7</sup>*Department of Electrical and Computer Engineering,  
Northwestern University, Evanston, IL 60208, USA*

## CONTENTS

|                                                      |   |
|------------------------------------------------------|---|
| I. Spectral Properties of Thin Film and Bilayer VOPc | 2 |
| II. Materials Characterization of VOPc Film          | 3 |
| III. DFT and TDDFT Calculations                      | 4 |

---

\* These authors contributed equally

† n-stern@northwestern.edu

# I. SPECTRAL PROPERTIES OF THIN FILM AND BILAYER VOPC

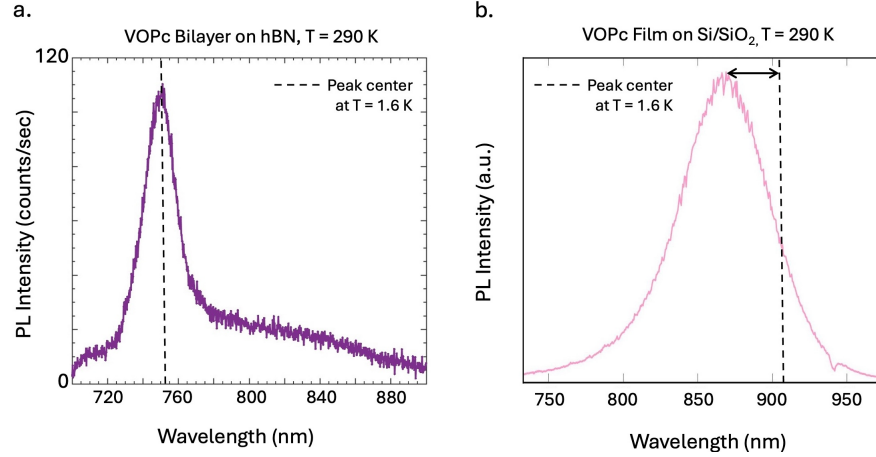

FIG. S1. (a) PL spectra of bilayer VOPc on hBN at room temperature (RT). The black dashed line indicates the center wavelength of the peak at cryogenic temperatures, demonstrating that there is negligible spectral shift. However, the count rate of the RT emission is much lower, with the maximum peak intensity reaching only about 110 counts/sec as opposed to almost 2500 counts/sec at  $T = 1.6$  K. (b) PL spectra of thicker film VOPc on Si/SiO<sub>2</sub> at RT; the black dashed line indicates the peak center of its  $T = 1.6$  K counterpart. At RT, VOPc emission from unordered molecules is shifted approximately 45 nm, or about 60 meV. Unlike 2D semiconductors, which blueshift when temperature decreases, VOPc molecules blueshift when temperature increases.

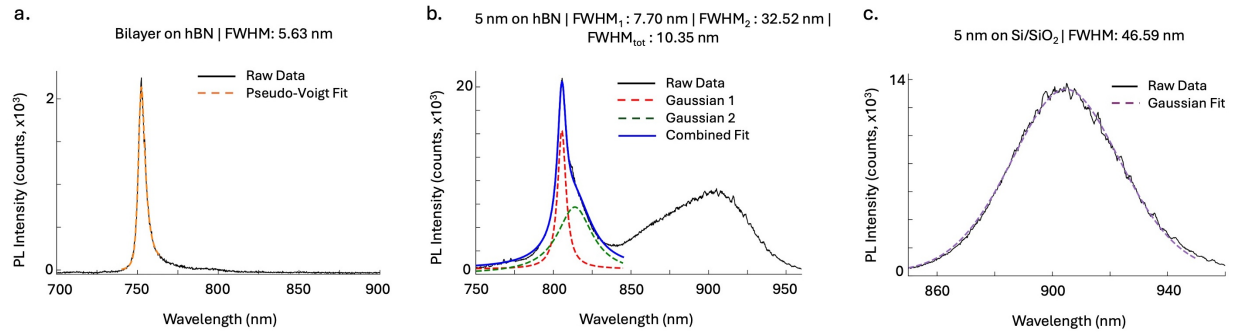

FIG. S2. Fitted peak data and full width half max (FWHM) for all iterations of VOPc PL, demonstrating a  $\sim 8\times$  reduction in VOPc peak width between a single bilayer on hBN and the amorphous molecules on Si/SiO<sub>2</sub>. (a) Pseudo-Voigt peak fit for emission of bilayer VOPc on hBN; the extracted FWHM is 5.63 nm. (b) Combined Gaussian fit of 5 nm film VOPc on hBN; the combined FWHM is 10.35 nm. (c) Single Gaussian fit of 5 nm film VOPc on substrate; the FWHM is 46.59 nm.

## II. MATERIALS CHARACTERIZATION OF VOPC FILM

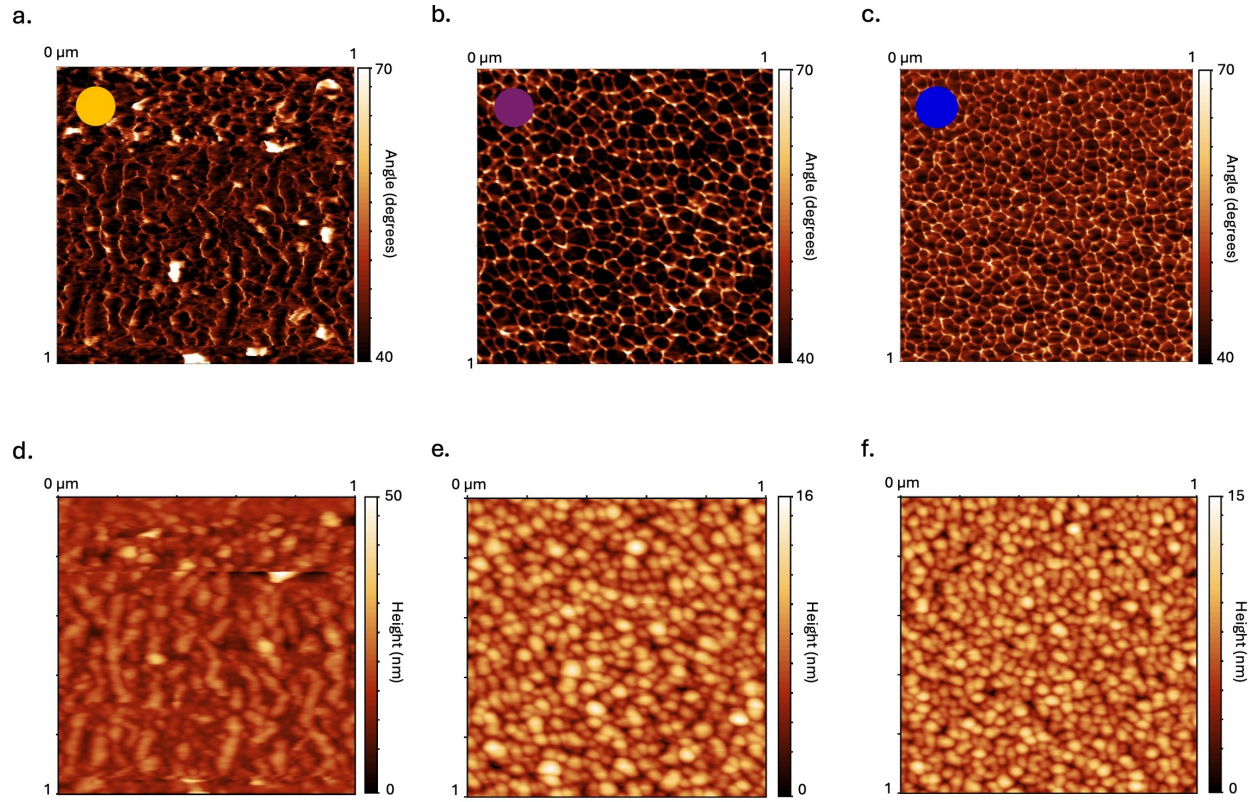

FIG. S3. Height AFM corresponding to the phase AFM from Figure 1. (a)-(c) Phase AFM of substrate, thin hBN, and thick hBN, respectively. (d)-(f) Height AFM of (a)-(c), respectively.

### III. DFT AND TDDFT CALCULATIONS

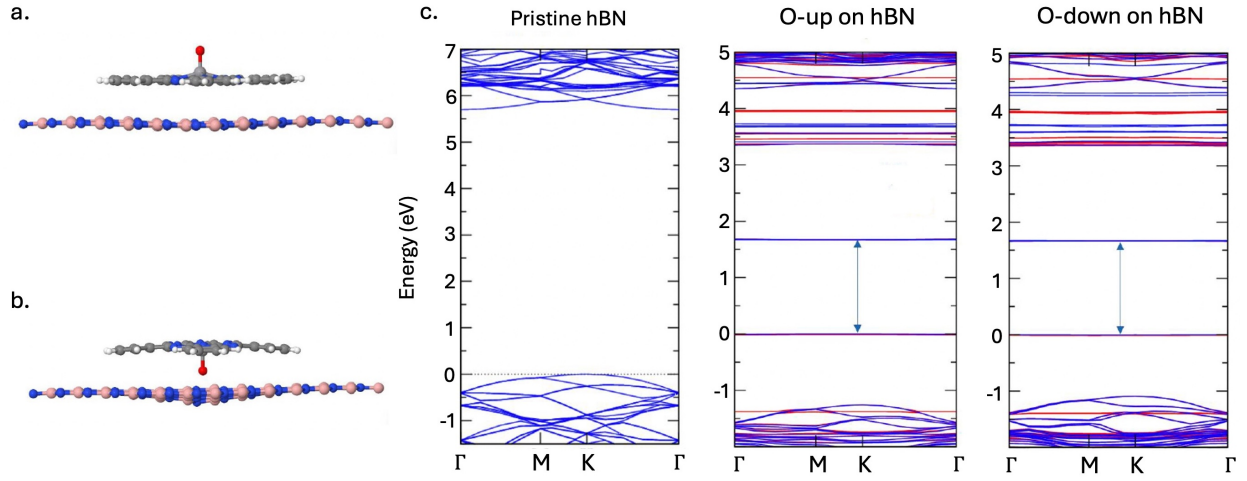

FIG. S4. (a) Schematic of VOPc in the O-up orientation on hBN. (b) Schematic of VOP in the O-down orientation on hBN. (c) DFT calculations of pristine hBN and both VOPc configurations; there is no difference in the VOPc gap magnitude (indicated by the arrow) solely based on orientation of the oxygen near the vdW surface.

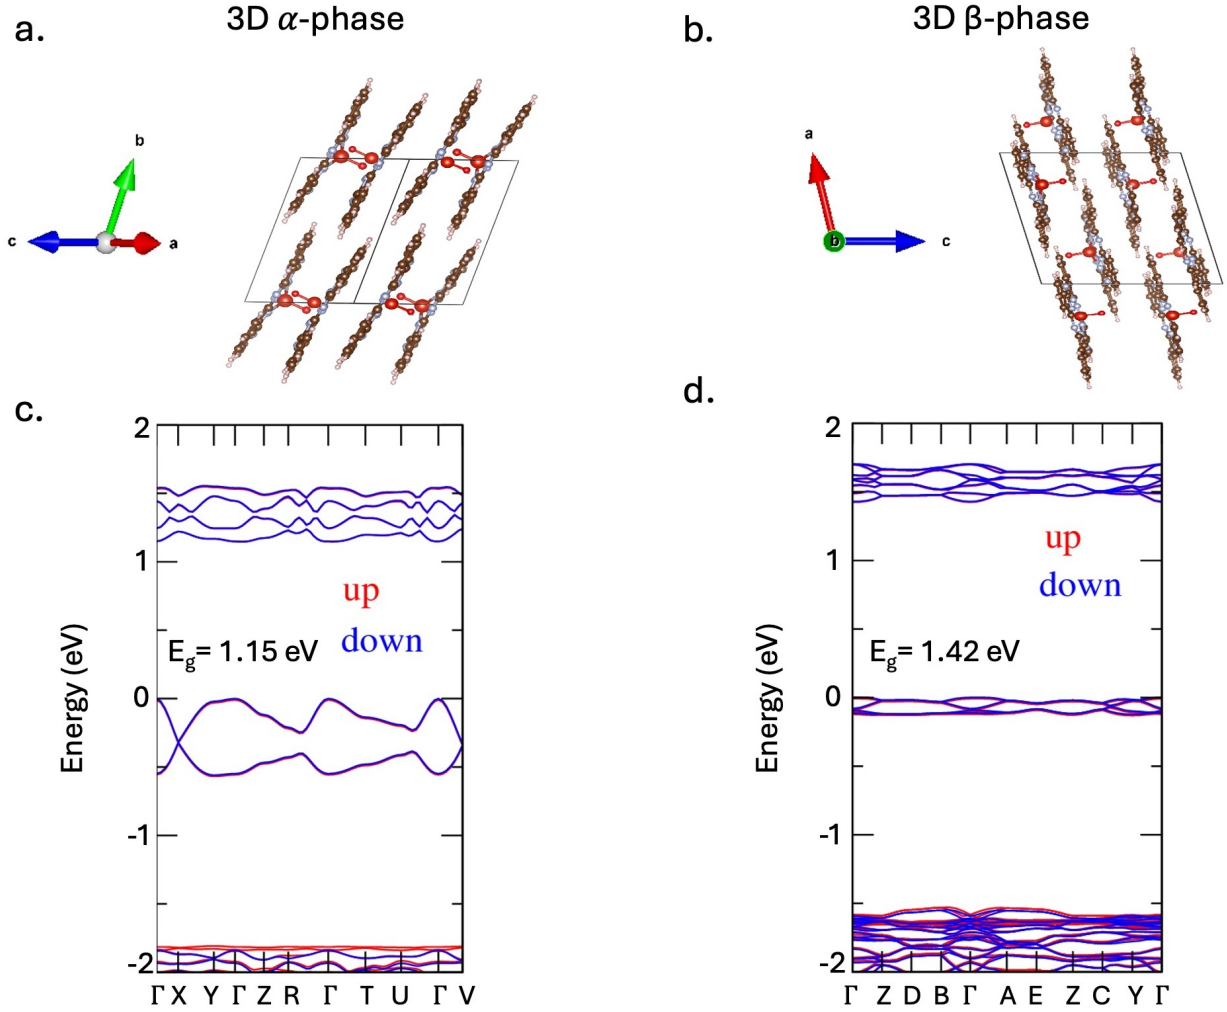

FIG. S5. 3D Configurations of VOPc. (a) Unit cell of alpha phase molecules in 3D. The triclinic unit cell lattice parameters corresponding to the vectors shown are the lattice constants  $a = 12.195$ ,  $b = 12.650$ , and  $c = 8.620$ , and the angles between them  $\alpha = 96.271$ ,  $\beta = 95.382$ , and  $\gamma = 68.040$ . (b) Unit cell of beta phase molecules in 3D. The monoclinic unit cell lattice parameters corresponding to the vectors shown are the lattice constants  $a = 13.778$ ,  $b = 13.353$ , and  $c = 13.990$ , and the angles between them  $\alpha = 90.0$ ,  $\beta = 103.614$ , and  $\gamma = 90.0$ . (c) and (d) Corresponding band structures of 3D alpha and beta phase molecules. The alpha phase band gap is smaller by about 270 meV.

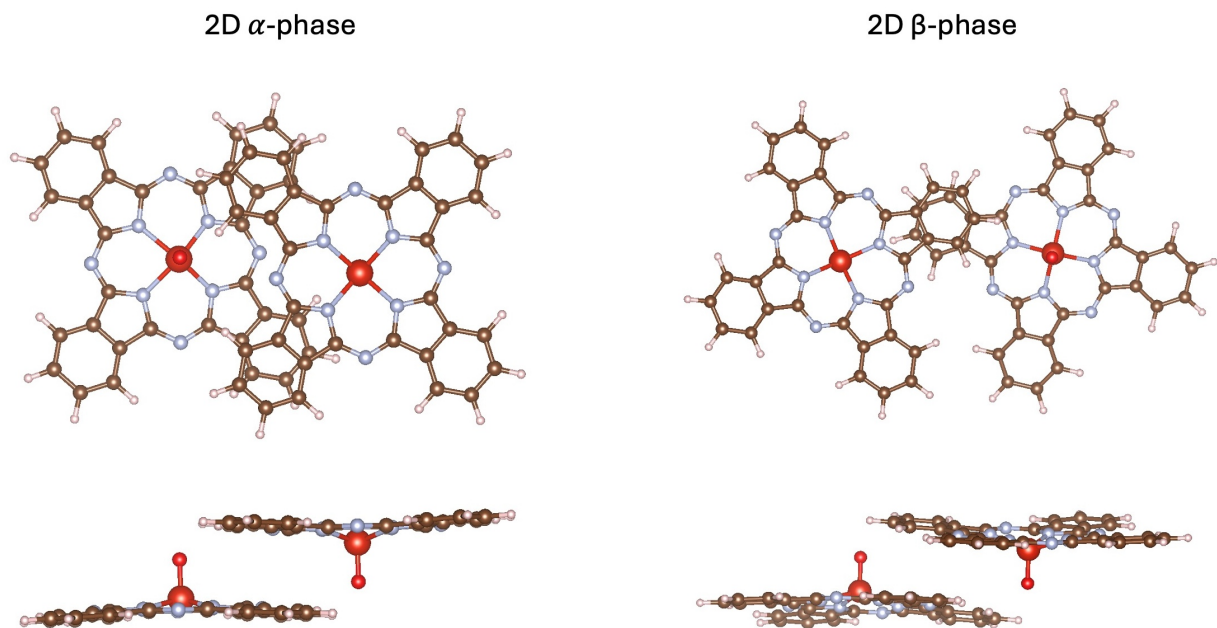

FIG. S6. Schematics of the phases of the excited state calculations performed in Table S1. In the alpha phase, the distance between two vanadium atoms is 7.46 Å and the distance between two macrocyclic rings is 3.25 Å. In the beta phase these are 10.34 Å and 3.28 Å, respectively.

| State        | Energy (eV) | Oscillator Strength | Character                  |
|--------------|-------------|---------------------|----------------------------|
| <b>Alpha</b> |             |                     |                            |
| 1            | 1.05056     | 0.00000263          | Pc to Pc                   |
| 2            | 1.07393     | 0.00000969          | Pc to Pc                   |
| 3            | 1.08000     | 0.00001365          | Pc to Pc                   |
| 4            | 1.09981     | 0.00000065          | Pc to Pc                   |
| 5            | 1.70024     | 0.00062305          | Pc to Pc                   |
| 6            | 1.74548     | 0.09635002          | Pc to Pc                   |
| 7            | 1.75312     | 0.01674481          | Pc to Pc                   |
| 8            | 1.76220     | 0.05897729          | Pc to Pc                   |
| 9            | 1.77019     | 0.00499714          | Pc to Pc                   |
| 10           | 1.77963     | 0.00112919          | Pc to Pc                   |
| 11           | 1.78155     | 0.00336444          | Pc to Pc                   |
| 12           | 1.79361     | 0.00023485          | Pc to Pc                   |
| 13           | 1.95910     | 0.00508378          | M to Pc and M+Pc; Pc to Pc |
| 14           | 1.96462     | 0.00535302          | Pc to Pc; M to Pc and M+Pc |
| 15           | 1.99322     | 0.00169972          | M to Pc, M+Pc              |
| 16           | 1.99908     | 0.63205662          | Pc to Pc                   |
| 17           | 2.04675     | 0.06020143          | Pc to Pc                   |
| 18           | 2.06716     | 0.53770732          | Pc to Pc                   |
| 19           | 2.31312     | 0.00011374          | M to Pc and M+Pc           |
| 20           | 2.32523     | 0.00010574          | M to Pc and M+Pc           |
| <b>Beta</b>  |             |                     |                            |
| 1            | 1.08957     | 0.00000353          | Pc to Pc                   |
| 2            | 1.09623     | 0.00000368          | Pc to Pc                   |
| 3            | 1.10702     | 0.00000623          | Pc to Pc                   |
| 4            | 1.10769     | 0.00000602          | Pc to Pc                   |
| 5            | 1.83006     | 0.00533839          | Pc to Pc                   |
| 6            | 1.83501     | 0.00111372          | Pc to Pc                   |
| 7            | 1.83656     | 0.00230715          | Pc to Pc                   |
| 8            | 1.84073     | 0.00109358          | Pc to Pc                   |
| 9            | 1.88744     | 0.00596454          | Pc to Pc                   |
| 10           | 1.89240     | 0.01555029          | Pc to Pc                   |
| 11           | 1.89454     | 0.00106602          | Pc to Pc                   |
| 12           | 1.90040     | 0.00393939          | Pc to Pc                   |
| 13           | 1.99357     | 0.70102794          | Pc to Pc                   |
| 14           | 2.01332     | 0.22306837          | Pc to Pc                   |
| 15           | 2.04603     | 0.54356155          | Pc to Pc                   |
| 16           | 2.06942     | 0.10433784          | Pc to Pc                   |
| 17           | 2.31846     | 0.00008201          | M to Pc and M+Pc           |
| 18           | 2.31947     | 0.00007881          | M to Pc and M+Pc           |
| 19           | 2.32711     | 0.00007462          | M to Pc and M+Pc           |
| 20           | 2.32966     | 0.00007875          | M to Pc and M+Pc           |

TABLE S1. Excited state calculations of VOPc and their character. ‘Pc to pc’ refers to transitions involving only the phthalocyanine ring. ‘M to Pc’ refers to transitioms from metal to phthalocyanine ring. ‘M + Pc’ refers to transitions of the metal plus phthalocyanine ring, aka the total VOPc molecule. Transitions with the highest oscillator strengths for both alpha and beta phases are highlighted in **red**.
